# Supplementary material for: QERA: an Analytical Framework for Quantization Error Reconstruction
Source: arXiv:2410.06040 source file (2025-02-15)
Supplement: Supplementary file 1 [file 999_appendix_qera_complexity.tex]

\subsection{Complexity Analysis}
\label{sec:appendix:complexity-analysis}

\tbgray{@Reviwer KXUq}, \tbpink{@Reviewer 1yFJ}

\tblue{We briefly analyze the computational complexity and memory complexity of QERA-exact and QERA-approx against LoftQ.
    ~\Cref{tab:appendix:time-complexity-qera-exact},~\Cref{tab:appendix:time-complexity-qera-approx},
    and~\Cref{tab:appendix:time-complexity-qera-loftq} summarize the computational complexity of QERA-exact, QERA-approx, and LoftQ, respectively.
    ~\Cref{tab:appendix:space-complexity-qera-exact},~\Cref{tab:appendix:space-complexity-qera-approx},
    and~\Cref{tab:appendix:space-complexity-loftq} summarize the memory complexity of QERA-exact, QERA-approx, and LoftQ, respectively.
    We notice that QERA-exact has the highest computational complexity and memory complexity.
    QERA-approx has a lower computational complexity but requires more memory footprint than LoftQ.
}

\begin{table}[h]
    \color{blue}
    \caption{Computational complexity of \loqerrxx{} of a linear layer. $(m,n)$ are the input and output feature sizes,
        $k$ denotes the rank, and $b$ is the number of calibration samples.}
    \centering
    \begin{footnotesize}
        \begin{tabular}{@{}ll@{}}
            \toprule
            Operation                              & Complexity             \\ \midrule
            Auto-correlation matrix $\mR_{\sX\sX}$ & $O(bm^2)$              \\
            Matrix square root of $\mR_{\sX\sX}$   & $O(m^3)$               \\
            Inverse of $\mR_{\sX\sX}^\frac{1}{2}$  & $O(m^3)$               \\
            SVD on weight matrix                   & $O(mn\cdot\min(m, n))$ \\
            Product to form $\mC_k$                & $O(m^3)$               \\
            \bottomrule
        \end{tabular}
    \end{footnotesize}
    \label{tab:appendix:time-complexity-qera-exact}
\end{table}
\begin{table}[h]
    \color{blue}
    \caption{Computational complexity of \loqerdiag{}. $(m,n)$ are the input and output feature sizes,
        $k$ denotes the rank, and $b$ is the number of calibration samples.}
    \centering
    \begin{footnotesize}
        \begin{tabular}{@{}ll@{}}
            \toprule
            Operation               & Complexity             \\ \midrule
            Scale matrix $\mS$      & $O(m^2\log_2 m)$       \\
            SVD on weight matrix    & $O(mn\cdot\min(m, n))$ \\
            Product to form $\mC_k$ & $O(m^3)$               \\ \bottomrule
        \end{tabular}
    \end{footnotesize}
    \label{tab:appendix:time-complexity-qera-approx}
\end{table}
\begin{table}[h]
    \color{blue}
    \caption{Computational complexity of \loftq{}. $(m,n)$ are the input and output feature sizes,
        $k$ denotes the rank, and $t$ is the iteration number.}
    \centering
    \begin{footnotesize}
        \begin{tabular}{@{}ll@{}}
            \toprule
            Operation               & Complexity              \\ \midrule
            Update quantized weight & $O(tmnk)$               \\
            Residual subtraction    & $O(tmn)$                \\
            SVD on weight matrix    & $O(tmn\cdot\min(m, n))$ \\ \bottomrule
        \end{tabular}
    \end{footnotesize}
    \label{tab:appendix:time-complexity-qera-loftq}
\end{table}
\begin{table}[h]
    \color{blue}
    \caption{Memory complexity of \loqerrxx{} of a linear layer. $(m,n)$ are the input and output feature sizes,
        $k$ denotes the rank, and $b$ is the number of calibration samples.}
    \centering
    \begin{footnotesize}
        \begin{tabular}{@{}lll@{}}
            \toprule
            Phase                         & Operation                                       & Complexity    \\ \midrule
            \multirow{2}{*}{Calibration}  & GEMM of linear forward pass                     & $O(bm+mn+bn)$ \\
                                          & Partial sum of $\mR_{\sX\sX}$                   & $O(m^2)$      \\ \midrule
            \multirow{6}{*}{Quantization} & Full-precision weight matrix                    & $O(mn)$       \\
                                          & Quantized weight matrix                         & $O(mn)$       \\
                                          & SVD on the scaled weight matrix                 & $O(mn)$       \\
                                          & Matrix square root of $\mR_{\sX\sX}$            & $O(m^2)$      \\
                                          & Matrix Inverse of $({\mR_{\sX\sX}}^{1/2})^{-1}$ & $O(m^2)$      \\
                                          & Low-rank terms                                  & $O(mk+nk)$    \\ \bottomrule
        \end{tabular}
    \end{footnotesize}
    \label{tab:appendix:space-complexity-qera-exact}
\end{table}

\tblue{In~\Cref{tab:appendix:runtime-qera-approx-vs-loftq}, we show a runtime comparison between QERA-approx and LoftQ (5-iter) since these two are designed for QPEFT experiments
    and the runtime (calibration + quantization time) should be in a reasonable range. We profile the runtime across various model sizes (1B, 3B, 7B, 13B, 30B)
    and find that QERA-approx is faster than LoftQ by 2-4 times. We attribute the larger overhead of LoftQ to two factors:
    1) The iterative SVD in LoftQ, an operation with the complexity $O(tmn\cdot \min(m,n))$ per layer,
    is performed for all linear layers. In contrast, QERA-approx only performs the SVD once per layer.
    2) In each iteration, LoftQ updates both the weights and low-rank terms.
    This requires around $O(tmn)$ memory read and store per layer between the GPU's global memory and local memory.
    For LLMs, this memory movement is bottlenecked by the limited bandwidth between HBM and SRAM.
    In contrast, QERA only calculates the low-rank terms,
    which means one $O(mn)$ read for weights and one $O((m+n)k)$ write
    where the rank value $k$ is very small ($k\ll \text{min}(m,n)$)
}

\begin{table}[h]
    \color{blue}
    \caption{Memory complexity of \loqerdiag{} of a linear layer. $(m,n)$ are the input and output feature sizes,
        $k$ denotes the rank, and $b$ is the number of calibration samples.}
    \centering
    \begin{small}
        \begin{tabular}{@{}lll@{}}
            \toprule
            Phase                         & Operation                       & Complexity    \\ \midrule
            \multirow{2}{*}{Calibration}  & GEMM of linear forward pass     & $O(bm+mn+bn)$ \\
                                          & Partial sum of $\mS$            & $O(m)$        \\ \midrule
            \multirow{5}{*}{Quantization} & Full-precision weight matrix    & $O(mn)$       \\
                                          & Quantized weight matrix         & $O(mn)$       \\
                                          & SVD on the scaled weight matrix & $O(mn)$       \\
                                          & Inverse of $\mS$                & $O(m)$        \\
                                          & Low-rank terms                  & $O(mk+nk)$    \\ \bottomrule
        \end{tabular}
    \end{small}
    \label{tab:appendix:space-complexity-qera-approx}
\end{table}
\begin{table}[]
    \color{blue}
    \caption{Memory complexity of \loqerdiag{} of a linear layer. $(m,n)$ are the input and output feature sizes,
        $k$ denotes the rank.}
    \centering
    \begin{footnotesize}
        \begin{tabular}{@{}lll@{}}
            \toprule
            Phase                         & Operation                       & Complexity \\ \midrule
            \multirow{4}{*}{Quantization} & Full-precision weight matrix    & $O(mn)$    \\
                                          & Quantized weight matrix         & $O(mn)$    \\
                                          & SVD on the scaled weight matrix & $O(mn)$    \\
                                          & Low-rank terms                  & $O(mk+nk)$ \\ \bottomrule
        \end{tabular}
    \end{footnotesize}
    \label{tab:appendix:space-complexity-loftq}
\end{table}
\begin{table}[]
    \color{blue}
    \caption{Runtime comparison of \loftq{} (5-iter) and \loqerdiag{} across various model sizes.
        For \loftq{} the runtime denotes the quantization time,
        while for \loqerdiag{} it denotes the calibration time plus the quantization time.
        \loqerdiag{} is faster than \loftq{} by 2-4 times. \tbgreen{@Reviwer 8w8V}}
    \centering
    \begin{small}
        \begin{tabular}{@{}lccccc@{}} \toprule
            Method      & 1B          & 3B           & 7B           & 13B          & 30B          \\ \midrule
            LoftQ       & 170s        & 1037s        & 3068s        & 7084s        & 45361s       \\
            QERA-approx & 70s         & 264s         & 738s         & 1952s        & 12495s       \\
            Speed up    & 2.4$\times$ & 3.94$\times$ & 4.16$\times$ & 3.63$\times$ & 3.62$\times$ \\ \bottomrule
        \end{tabular}
    \end{small}
    \label{tab:appendix:runtime-qera-approx-vs-loftq}
\end{table}
